# Supplementary material for: Greedy Output Approximation: Towards Efficient Structured Pruning for LLMs Without Retraining
Source: arXiv:2407.19126 source file (2024-07-26)
Supplement: Supplementary file 1 [file b-appendix.tex]

% \section{Appendix-B}

% \subsection{Pruning Individual Channels of Attention Head}
